# Supplementary material for: Many-Body Expanded Full Configuration Interaction. I. Weakly Correlated Regime
Source: arXiv:1807.01328 ancillary file (2018-10-15)
Supplement: Supplementary file 1 [file si.pdf]

# Supporting information for:

# Many-Body Expanded Full Configuration Interaction. I. Weakly Correlated Regime

Janus J. Eriksen* and Jürgen Gauss*

*Institut für Physikalische Chemie, Johannes Gutenberg-Universität Mainz, Duesbergweg 10-14, 55128 Mainz, Germany*

E-mail: jeriksen@uni-mainz.de; gauss@uni-mainz.de

*To whom correspondence should be addressed

# 1 CCSDTQ and SHCI

All CCSDTQ calculations in MRCC used an energy convergence threshold of $\delta E = 1.0 \times 10^{-9}\ E_{\mathrm{H}}$.

For all SHCI calculations in DICE, the following parameters—motivated by the defaults and numerical results of S. Sharma *et al.*: JCTC **13**, 1595 (2017)—were used:
$\delta E = 1.0 \times 10^{-9}\ E_{\mathrm{H}}$, $\varepsilon_1 = 5.0 \times 10^{-4}\ E_{\mathrm{H}}$, $\varepsilon_2^d = 5.0 \times 10^{-6}\ E_{\mathrm{H}}$, $\varepsilon_2 = 5.0 \times 10^{-8}\ E_{\mathrm{H}}$, $N_d = 200$, and a target standard deviation of the semistochastic corrected energy of $1.0 \times 10^{-4}\ E_{\mathrm{H}}$ (default value). Due to the fact that SHCI electronic energies from the DICE program are returned with associated statistical error bars due to the stochastic sampling, all results of the present work have been obtained as average values from five successive runs (averaging both energies and error bars).

# 2 Geometries and Reference Energies

All geometries and reference energies are given in atomic units.

Table S1: $H_2O$ — $C_{2\mathrm{v}}$

| Atom | $x$ | $y$ | $z$ |
|---|---|---|---|
| H | 0.00000000 | −1.42467141 | 0.98653069 |
| O | 0.00000000 | 0.00000000 | −0.12432080 |
| H | 0.00000000 | 1.42467141 | 0.98653069 |

Table S2: $H_2O$ — $C_{2\mathrm{v}}$

| Basis set | HF | CCSD | CCSD(T) |
|---|---|---|---|
| cc-pVDZ | −76.026853 | −76.237991 | −76.240915 |
| cc-pVTZ | −76.057222 | −76.324553 | −76.332556 |
| cc-pVQZ | −76.064889 | −76.350810 | −76.360326 |

Table S3: (Be–He) and $(\text{Be–He})_2$ — $C_{\infty\text{v}}$

| Atom | $x$ | $y$ | $z$ |
|---|---|---|---|
| | | Be–He | |
| Be | 0.00000000 | 0.00000000 | 2.362157665 |
| He | 0.00000000 | 0.00000000 | −2.362157665 |
| | | He–Be···Be–He | |
| He | 0.00000000 | 0.00000000 | 193.69691564 |
| Be | 0.00000000 | 0.00000000 | 188.97261920 |
| Be | 0.00000000 | 0.00000000 | −188.97260758 |
| He | 0.00000000 | 0.00000000 | −193.69694181 |

Table S4: (Be–He) and $(\text{Be–He})_2$ — $C_{\infty\text{v}}$

| Basis set | HF | CCSD | CCSD(T) |
|---|---|---|---|
| | | Be–He | |
| cc-pVDZ/STO-3G | −17.374136 | −17.420487 | −17.420551 |
| | | He–Be···Be–He | |
| cc-pVDZ/STO-3G | −34.748272 | −34.840975 | −34.841102 |

Table S5: $C_2H_4$ — $D_{2h}$

| Atom | $x$ | $y$ | $z$ |
|---|---|---|---|
| | | Zimmerman | |
| C | 1.25306582 | 0.00000000 | 0.00000000 |
| C | −1.25306582 | 0.00000000 | 0.00000000 |
| H | 2.31052152 | 1.73913172 | 0.00000000 |
| H | 2.31052152 | −1.73913172 | 0.00000000 |
| H | −2.31052152 | −1.73913172 | 0.00000000 |
| H | −2.31052152 | 1.73913172 | 0.00000000 |
| | | Daday *et al.* | |
| C | 1.25633907 | 0.00000000 | 0.00000000 |
| C | −1.25633907 | 0.00000000 | 0.00000000 |
| H | 2.31647921 | −1.74281127 | 0.00000000 |
| H | 2.31647921 | 1.74281127 | 0.00000000 |
| H | −2.31647921 | −1.74281127 | 0.00000000 |
| H | −2.31647921 | 1.74281127 | 0.00000000 |

Table S6: $C_2H_4$ — $D_{2h}$

| Basis set | HF | CCSD | CCSD(T) |
|---|---|---|---|
| | | Zimmerman | |
| ANO-L-VDZP | −78.054899 | −78.349573 | −78.359303 |
| | | Daday *et al.* | |
| ANO-L-VDZP | −78.054933 | −78.350050 | −78.359840 |

Table S7: $CH_2$ — $C_{2v}$

| Atom | $x$ | $y$ | $z$ |
|---|---|---|---|
| H | 0.00000000 | −1.86931709 | 0.69109398 |
| C | 0.00000000 | 0.00000000 | −0.11608364 |
| H | 0.00000000 | 1.86931709 | 0.69109398 |

Table S8: $CH_2$ — $C_{2v}$

| Basis set | HF | CCSD | CCSD(T) |
|---|---|---|---|
| cc-pVDZ | −38.921509 | −39.039561 | −39.041358 |
| cc-pVTZ | −38.932221 | −39.074329 | −39.077982 |

Table S9: $O_2$ — $D_{\infty h}$

| Atom | $x$ | $y$ | $z$ |
|---|---|---|---|
| O | 0.00000000 | 0.00000000 | 1.14094105 |
| O | 0.00000000 | 0.00000000 | −1.14094105 |

Table S10: $O_2$ — $D_{\infty h}$

| Basis set | HF | CCSD | CCSD(T) |
|---|---|---|---|
| cc-pVDZ | −149.608081 | −149.974818 | −149.985703 |
